# Supplementary material for: Tuning insulator-semimetal transitions in 3D topological insulator thin films by inter-surface hybridization and in-plane magnetic fields
Source: arXiv:1904.03722 source file (2019-04-07)
Supplement: Supplementary file 1 [file Supplementary_information.pdf]

# Supplementary Information

## I. Effect of an in-plane magnetic field on the surface states of a 3D TI

The basic theoretical model we use has been explained in ref. [1]. Here we present a detailed derivation and show how to understand the gap closing mechanism intuitively. Furthermore, we show how adding a quadratic term (not included in ref. [1]) to the Hamiltonian may affect the results.

The effective model of the Hamiltonian for the massless Dirac fermions of a 3D topological insulator surface state writes:

$$H = \hbar v_F(\hat{z} \times \boldsymbol{\sigma}) \cdot \boldsymbol{k}, \qquad (1)$$

where $\hbar$ is the reduced plank constant, $v_F$ is the Fermi velocity, $\hat{z} = (0, 0, 1)$ is the unit vector normal to the surface, $\boldsymbol{\sigma} = (\sigma_x,\ \sigma_y,\ \sigma_z)$ is the Pauli matrices (for the real spin) and $\boldsymbol{k} = (k_x, k_y, k_z)$ is the wavevector. The corresponding gapless Dirac band ($\varepsilon = \pm\hbar v_F|\boldsymbol{k}|$) for the surface states of a 3D TI film has a helical spin-momentum locking structure. As long as the film is thick enough and the time reversal symmetry is preserved, the two massless Dirac cones remain intact.

However, when a 3D TI film is thin enough, the tunneling (or so called hybridization) between the top and bottom surfaces must be considered. The thin TI system can be modeled by a surface state Hamiltonian which has the following form:

$$H = \hbar v_F \tau_z(\hat{z} \times \boldsymbol{\sigma}) \cdot \boldsymbol{k} + \Delta\tau_x, \qquad (2)$$

in the basis of $|u\uparrow>$, $|u\downarrow>$, $|d\uparrow>$ and $|d\downarrow>$, where the top and bottom surfaces can be considered as pseudospins ($u$ and $d$, respectively) with corresponding Pauli matrices $\tau_i$ ($i$=x, y, z), $\uparrow$ and $\downarrow$ represent the real spin up and down states and $\Delta$ is the tunneling term in the zeroth order approximation (the identity matrix in the real spin space is implicit in the $\Delta\tau_x$ term). The band acquires a massive Dirac dispersion $\varepsilon = \pm\sqrt{(\hbar v_F \boldsymbol{k})^2 + (\Delta_0/2)^2}$, where $\Delta_0 = 2\Delta$ is the gap size.

Consider a thin 3D TI film with the top and bottom surfaces located at $z = \pm t/2$, where $t$ is the film thickness. Assume the film is subject to a magnetic field $\boldsymbol{B} = B\hat{x}$ parallel to the film

surface and in the x direction, we can introduce a vector potential $\boldsymbol{A} = -Bz\hat{y}$ to the kinetic momentum $\hbar\boldsymbol{k} + e\boldsymbol{A}$. Now the TI surface state Hamiltonian becomes:

$$H = v_F\tau_z(\hat{z} \times \boldsymbol{\sigma}) \cdot \left(\hbar\boldsymbol{k} - \frac{\tau_z eBt\hat{y}}{2}\right) + g\mu_B\sigma_x B/2 + \Delta\tau_x, \quad (3)$$

where $g\mu_B\sigma_x B/2$ is the Zeeman energy term with $g$ (which would be ≈2 in free space) being the in-plane g-factor for the topological surface states and $\mu_B$ is the Bohr magneton. Since $\sigma_x B = (\hat{z} \times \boldsymbol{\sigma}) \cdot B\hat{y}$, the Hamiltonian can be simplified as:

$$H = v_F\tau_z(\hat{z} \times \boldsymbol{\sigma}) \cdot [\hbar\boldsymbol{k} - \tau_z(\frac{et}{2} - \frac{g\mu_B}{2v_F})B\hat{y}] + \Delta\tau_x, \quad (4)$$

which corresponds to a $4 \times 4$ matrix:

$$\begin{pmatrix} 0 & [ik_x + (k_y - \kappa_B)]\hbar v_F & \Delta & 0 \\ [-ik_x + (k_y - \kappa_B)]\hbar v_F & 0 & 0 & \Delta \\ \Delta & 0 & 0 & -[ik_x + (k_y + \kappa_B)]\hbar v_F \\ 0 & \Delta & -[-ik_x + (k_y + \kappa_B)]\hbar v_F & 0 \end{pmatrix}$$

with a magnetic wavevector $\kappa_B = \left(\frac{et}{2} - \frac{g\mu_B}{2v_F}\right) B/\hbar$. The spectrum of the Hamiltonian is given by:

$$\varepsilon = \pm\sqrt{(\hbar v_F)^2(k_x^2 + k_y^2 + \kappa_B^2) + \Delta^2 \pm 2(\hbar v_F\kappa_B)\sqrt{\Delta^2 + \left(\hbar v_F k_y\right)^2}}. \quad (5)$$

For non-zero $\Delta$, the surface band structure undergoes a quantum phase transition at a critical magnetic field $B = B_c$ satisfying $|\hbar v_F\kappa_B| = \Delta$. At $B < B_c$, the spectrum (shown in Fig. 4a and shown in Fig. S1a with two low-energy sub-bands attached with spin orientations) has solution $\varepsilon = \pm(\Delta \pm |\hbar v_F\kappa_B|)$ at $\boldsymbol{k} = 0$. Here the band is trivial with a band gap of $\Delta_B = \Delta_0 - |E_B|$, in which $E_B(= -2\hbar v_F\kappa_B = (g\mu_B - etv_F)B)$ defines an effective magnetic (Zeeman-like) energy. The two terms in $E_B$ correspond to the contributions from the actual Zeeman coupling and Aharonov-Bohm phase gradient, respectively. It can also be understood semiclassically as follows. For an electron moving around the circumference of a cross section (normal to $B$, see Fig. 4b) at velocity $v_F$, it gains extra energy from the magnetic field due to an orbital magnetic moment with magnitude of:

$$\mu_{orb} = I * S = \frac{e}{2(w+t)/v_F} * wt = \frac{wt}{2(w+t)} ev_F, \quad (6)$$

where $I$ is the current generated by the electron surrounding the loop with area $S$ (rectangular shape with sides $w$ and $t$) and $e$ is the elementary charge. In the limit of $w>>t$, which is satisfied in our BSTS samples (usually with $w$ a few μm and $t$ tens of nm or less), $\mu_{orb} = etv_F/2$. Due to the spin-momentum locking of the surface states, the electrons with clockwise and counter-clockwise motion possess opposite spin directions that are parallel and anti-parallel to $\boldsymbol{B}$ (Fig. 4b), thus having opposite total magnetic moments of $\mp(\frac{g\mu_B}{2} - \frac{etv_F}{2})$, respectively. This gives a splitting (Fig. 4a) of each band (into two sub-bands) with the magnetic field, where one sub-band shifts up in energy by $|(g\mu_B - etv_F)B/2|$, and the other sub-band shifts down by the same amount. A similar analysis applies for the hole band near the gap. Overall, the gap size decreases by an "effective energy" (acting like a Zeeman energy) $E_B = (g\mu_B - etv_F)B$. One can also define an effective g-factor $g_{eff} = \frac{E_B}{B\mu_B} = (g - etv_F/\mu_B)$ accordingly.

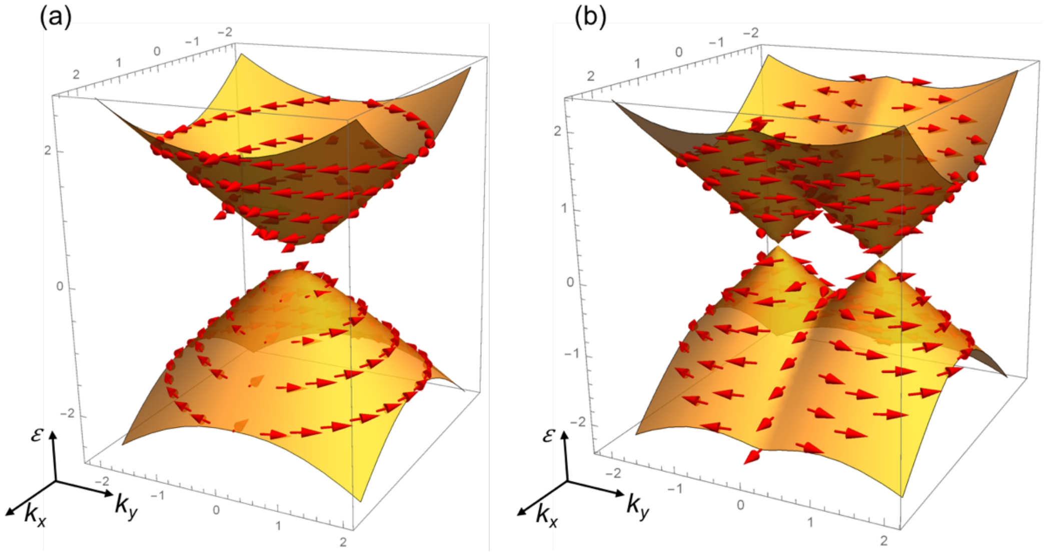


Fig. S1. (a) The two low-energy (with smallest | ε |) sub-bands from Equation (5) in the condition of 0<B<Bc. The red arrows denote spin direction. (e-h) Similar plots for the 2D topological semimetal phase at B>Bc, where the two Dirac cones are recovered and have opposite spin helicity. The units for axis are arbitrary.

At $B > B_c$, the spectrum (shown in Fig. 2G and shown in Fig. S1b with two low-energy sub-bands attached with spin orientations) becomes gapless and restores two Dirac cones separated in the momentum space along the $k_y$ direction. This gives an intriguing topological 2D semimetal phase induced by the large in-plane magnetic field.

For $\Delta = 0$, the band structure reduces to the case for thick films without hybridization:

$$\varepsilon = \pm\hbar v_F\sqrt{k_x^2 + (k_y \pm \kappa_B)^2}, \quad (7)$$

which simply implies two relatively shifted Dirac cones in momentum space at $k_y = \pm\kappa_B$.

We have also considered a more realistic band structure with a quadratic term $\frac{(\hbar k)^2}{2m^*}$ added to the Hamiltonian, with $m^*$ being the effective mass. It's found that only the Fermi velocity $v_F$ to the linear term $\hbar v_F \tau_z(\hat{z} \times \boldsymbol{\sigma}) \cdot \boldsymbol{k}$ contributes to the effective energy $E_B$. We estimated $m^* \approx 0.17 m_e$ and $v_F \approx 1.3 \times 10^5\ m/s$ from the angle-resolved photoemission spectroscopy measurements of bulk BSTS [2]. Based on that and the relatively small $|\frac{E_B}{B}|$ value extracted from experiment for Device N5, we estimate $g \approx \frac{etv_F}{\mu_B} \approx 20$.

## II. Sample preparation and measurement

TI single crystals $BiSbTeSe_2$ (BSTS) were grown by the vertical Bridgman technique [3]. The dual-gated BSTS devices were fabricated into Hall-bar structures on highly p-doped Si substrates (with 300 nm-thick $SiO_2$ coating) with hexagonal boron nitride (h-BN) flakes (tens of nm in thickness) transferred onto the devices as top-gate dielectrics. Similar fabrication procedures for the dual-gated BSTS devices have been described elsewhere [4].

Transport measurements are performed in a helium-4 variable temperature system (with base temperature down to 1.6 K) or helium-3 systems equipped with magnetic fields up to 18 T, 31 T or 45 T (down to 0.3 K). The magnetoresistance MR is defined as $(\rho(B) - \rho(0))/\rho(0)$, where $\rho(B)$ is the B-dependent resistivity. For all the transport measurements, Keithley 2400 source meters are used to apply gate voltages ($V_{tg}$ and $V_{bg}$). Depending on the maximum resistance ($R_{max}$) of a specific sample, we measure it in different ways for better accuracy. For the most insulating samples (like Device N4 with t=6 nm and $R_{max}$>>MΩ), we use two-terminal measurements. A constant AC (applied by Stanford SR830 lock-in with frequency <10 Hz) or DC (applied by Keithley 2400 source meter) source-drain voltage ($V$=100 mV or 10 mV) is applied across the sample while the current ($I$) is monitored to give conductance (=$I/V$). No measurable conductance or any gate tunability has been observed even at room temperature for BSTS flakes below ~5 nm,

so we didn't show any data for these flakes. For samples with $R_{max}$ less than a few MΩ (usually $t$≥8 nm), conventional four-terminal measurements with Hall bar structures (Fig. 1A) are used to measure the resistance. Generally, a low-frequency (<20 Hz) AC excitation current of 100 nA (when $R_{max}$<~100 kΩ), 1 nA (~100 kΩ<$R_{max}$<~1 MΩ) or 0.2 nA (~1 MΩ<$R_{max}$<~10 MΩ), where the current is reduced for larger $R_{max}$ to avoid self-heating effect, is applied by a SR830 lock-in amplifier (input impedance 10 MΩ). If ~100 kΩ<$R_{max}$<~10 MΩ, an extra voltage preamplifier (model DL 1201) with input impedance of 100 MΩ is added to improve the accuracy of voltage detection.

## III. More details of the zero-field transport measurements and discussion

We have performed temperature dependent measurements of multiple samples with various thicknesses. In Fig. S2a, we replotted four representative data sets from Fig. 2E as $\sigma_{min}$ (=1/$\rho_{max}$) versus 1/$T$, where $\sigma_{min}$ (or $\rho_{max}$) is reached when both the two surfaces are gated to Dirac point or charge neutrality point. For samples with $t$>~10 nm (e.g. $t$=14 nm), $\rho_{max}$(T) only shows metallic behavior ($d\rho_{max}/dT>0$) below ~50 K, indicating gapless surface states. The size of non-zero effective transport gap $\Delta_0^*$ in thinner BSTS samples is estimated from thermal activation fit with $\rho_{max}(T) \propto e^{\Delta_0^*/2k_BT}$ or $\sigma_{min}(T) \propto e^{-\Delta_0^*/2k_BT}$ in appropriate temperature ranges, beyond which other conduction mechanisms need to be considered to describe the temperature dependent conduction. For example, in samples with t=10 nm (Device N3 and N5) and 8 nm, the thermal activation fit has been applied to the temperature range between ~3 K to ~30 K, where an insulating behavior is observed, to extract $\Delta_0^*$ (note that it could be smaller than the real hybridization gap $\Delta_0$ due to smearing effect of potential fluctuations at different positions). This temperature range is chosen for the following reasons. Usually below 3 K, $\sigma_{min}$ tends to deviate from a single thermal activation fit. As shown in Fig. S2b of a typical example N5, we can fit the temperature dependent data down to 0.3 K with an empirical formula $\sigma_{min} = C_1 e^{-T_1/T} + C_2 e^{-(T_2/T)^{1/3}}$, which gives $T_1$=~8 K and $T_2$=~0.02 K. The second term has the form of variable range hopping (VRH) for 2D (we caution that other forms may be used that also give reasonable fits), suggesting multiple

conduction mechanisms at lower temperatures. Above ~30 K, Dirac points usually shift and the peak become much broader in gate-voltage sweeps (see Fig. S4a as a typical example), indicating additional conducting channels such as impurities or bulk states. In Fig. 4, a similar temperature range (3 K~25 K) has been used to fit the data of Device N5 under in-plane magnetic fields.

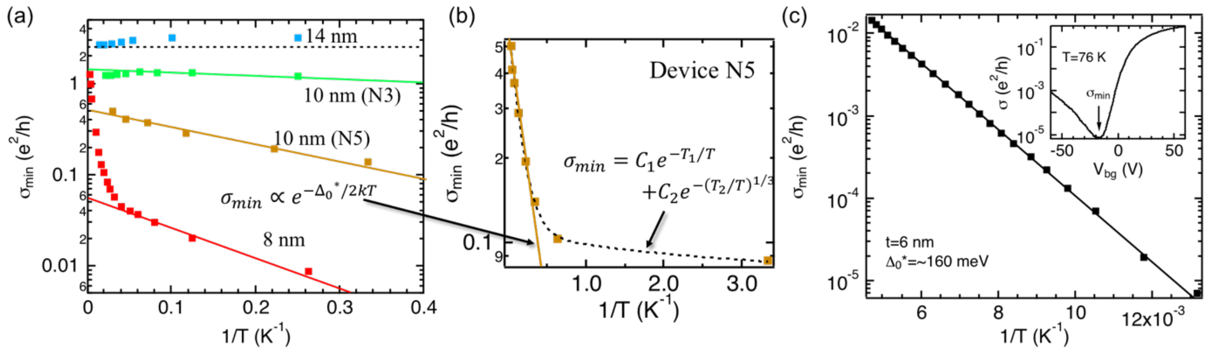


Fig. S2. (a) Same data from Fig.1h replotted as minimum conductivity $\sigma_{min}$ ($=1/\rho_{max}$) versus 1/T for four BSTS samples. The solid lines are the corresponding fittings from thermal activation $\sigma_{min}(T) \propto e^{-\Delta_0{}^*/2k_BT}$ for the thin samples (typically in the temperature range between 3 K to 30 K). The dashed horizontal line is a guide to the eye for a thicker (14 nm) sample showing an opposite trend (in $\sigma_{min}$ versus 1/T) compared to the thin ones, indicating a metallic behavior and a zero gap. (b) The $\sigma_{min}$ versus 1/T for Device N5 (10 nm thick) in a larger temperature range (down to 0.3 K). The yellow solid line is the same thermal activation fit in (a) for higher temperatures while the dashed curve is a fit based on the formula shown in the (b) for the whole temperature range. (c) In a 6-nm-thick sample, thermal activation fits well in the entire temperature range (76 K to 300 K), giving a gap size of ~160 meV. Inset is a typical back gate dependence for the 2-termial conductivity $\sigma$ measured at 76 K for this device.

In Fig. S2c, we showed the thermal activation fit for another 6 nm-thick device in the temperature range of 76 K to ~300 K, below which $\sigma_{min}$ becomes too small to be detected accurately due to limitation of our instruments. The good linearity of $\sigma_{min}$ in logarithmic scale versus 1/T indicates a hard gap opening in this device and the fitting gives a gap size ~160 meV, which is much larger than that determined by angle-resolved photoemission spectroscopy (ARPES) measurements on 6 nm $Bi_2Se_3$ grown by molecular beam epitaxy (surface gap barely vanishes at 6 nm) [5] and the theory prediction for $Bi_2Se_3$ (a few meV at 6 nm) [6] [7]. A much enhanced gap size has also reported previously on exfoliated $Bi_2Se_3$ thin flakes in ref. [8]. Given the material difference and better isolated surface conduction, the gap size in our thin BSTS films grows monotonically with reducing thickness and roughly follow an exponential function $\Delta_0{}^* \propto e^{-0.7[\frac{t}{(nm)}]}$ (Fig. 2F inset). We don't have evidence of oscillatory behavior of $\Delta_0{}^*$ versus t and did not observe any signs of quantum spin Hall effect [6] [7] [9].

The typical mobility of our sample with thickness ≥~10 nm is a few thousand cm$^2$/Vs, which can be referred in our previous publications (*3*). For Device N4 with thickness 6 nm, the mobility is reduced to less than 100 cm$^2$/Vs for both electron and hole doped sides. The scattering time τ of the samples can be estimated by $\tau = \hbar\sigma\left(\frac{2\pi}{n}\right)^{\frac{1}{2}}/(e^2 v_f)$ from Drude model and employing the Einstein relation. The corresponding mean free path can be obtained by $l = \tau v_f$, which ranges from 10~40 nm for typical samples (≥~10 nm thick).

## IV. Additional information for Device N5 (Fig. S3 to Fig. S6)

As seen in Fig. S3c, Device N5 (see device optical images in Fig. S3a and S3b) shows maximum resistivity $\rho_{max}$ near $V_{bg}$≈30 V and $V_{tg}$≈1 V (note that depending on gate sweep histories, the exact peak position could vary slightly) at zero field and base temperature T=0.3 K.

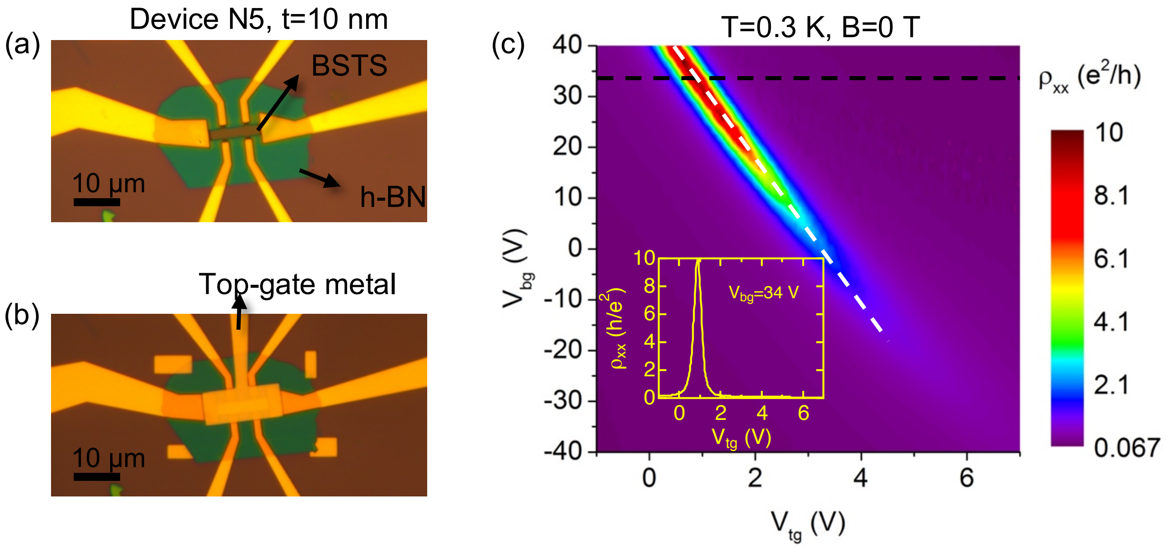


Fig. S3. (a,b) Optical images for the BSTS device N5 before and after top-gate metal deposition. The BSTS flake is etched into a Hall-bar structure and covered with a hexagonal boron nitride (h-BN) flake (~24 nm thick) as top-gate dielectric. (c) The four-terminal 2D resistivity $\rho_{xx}$ as a function of top and back gate voltages ($V_{tg}$ and $V_{bg}$) for Device N5. The behavior is similar to that of Device N3 with resistivity peak along the total charge neutral line (dashed white line). However, Device N5 is initially more n doped and has a larger $\rho_{max}$ (~10 h/e$^2$) as identified from the maximum resistivity peak in the line cut (shown in the inset) along the dashed line near $V_{bg}$=34 V.

Most of the data of N5 shown in the main text were taken in a hybrid magnet system (up to 45 T) at NHMFL (Tallahassee, FL), referred as "first cool down". During the experiments, we notice that adjusting both gates is time consuming and could easily cause hysteresis thus uncertainties in the doping level of the two surfaces. Instead, for consecutive measurements (at different temperatures and magnetic fields), we fix $V_{bg}$ at 30 V and identify the resistivity peak in top gate ($V_{tg}$) sweeps (always sweeping in the same range and same rate ~40 sec/V) as the global maximum resistivity $\rho_{max}$ (shown in Fig. 2f and 3a). We note that during the measurements of this set of data, the outer superconducting magnet of the hybrid magnet is maintained at 11.4 T and can not be changed. Fig. S4a and S4b show typical examples of these $V_{tg}$ sweeps. In Fig. S4a the in-plane magnetic field is maintained at 11.4 T while the temperature is varied. In Fig. S4b the magnetic field is varied (using the inner resistive magnet of the hybrid magnet) while the temperature is kept at 0.3 K. It confirms our general observation that neither the in-plane B field nor the temperature (below T~25 K) shifts the peak position (see also Fig. 2, Fig. S8 and Fig. S9). Therefore we can measure $\rho_{max}$ at fixed gate voltages by continuously changing in-plane B fields in Fig. 2f (note the outside superconducting magnet is shut down during this specific run, allowing the sweeping of both positive and negative magnetic fields up to ~34 T) and Fig. S5 (measured at different temperatures below ~25 K in a third cool down). The inset of Fig. S4a shows the typical configuration with in-plane field parallel to current direction for the measurements described in the main text and supplementary material. The only exceptions are Fig. S6 and Fig. S7 discussed below.

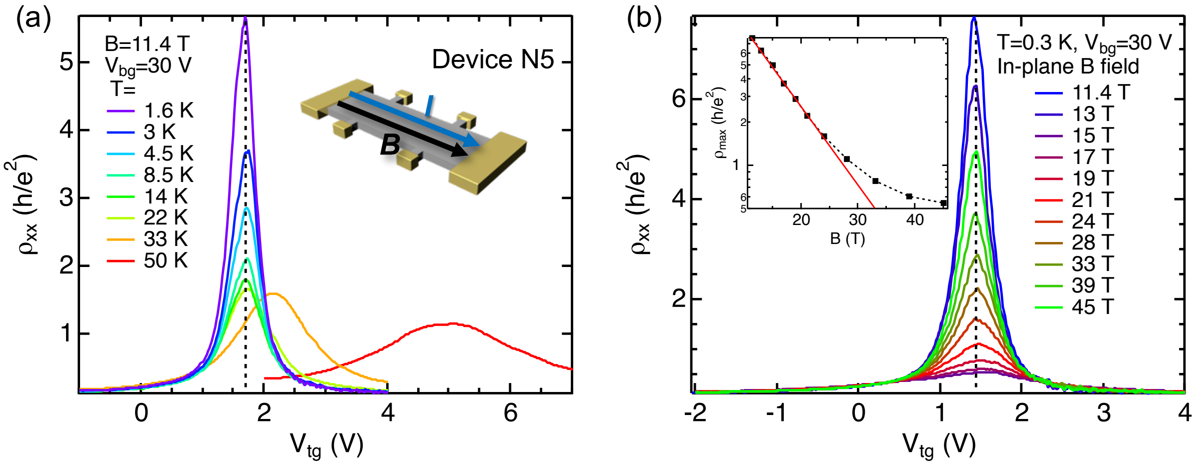


Fig. S4. The $\rho_{xx}$ as a function of top gate voltage $V_{tg}$ with fixed $V_{bg}$=30 V at (a) in-plane B=11.4 T and various temperatures and (b) (same data shown in Fig. 2e) different in-plane magnetic fields and $T$=0.3 K.

Below ~25 K, the corresponding $V_{tg}$ position of the resistivity peak is almost the same at ~1.7 V. Above ~25 K, the peak position deviates from the constant value ~1.7 V and the peak value is not used for the thermal activation fittings in Fig. 4. The inset of (a) shows the measurement configuration with the in-plane field parallel to the current (I) direction. The inset of (b) shows the $\rho_{max}$ (extracted from the peak values in b) in log scale as a function of the corresponding *B* field. The red solid line is a guide to the eye of the linear dependence of log($\rho_{max}$) with B below ~30 T. Above 30 T, $\rho_{max}$ tends to saturate towards $h/2e^2$.

Fig. S5 shows an additional set of measurements (referred as the third cool down) of the dependence of $\rho_{max}$ on the in-plane field B at different temperatures when both surfaces are tuned to charge neutrality points (fixed gate voltages). As shown in Fig. S5a, the low field features (below 5 T), including a cusp near B=0 and some positive MR, are both smeared out at T>6 K. The cusp feature was not observed in the less insulating sample N3, and could be attributed to quantum interference effect of VRH transport in a strong localization regime [10]. The positive MR may be related to the suppression of hopping transport due to spin polarization at localized states by moderate magnetic field (~5 T) [11]. In contrast, the negative MR shown at higher fields (>5 T) is much more robust at elevated temperatures (still pronounced at 27 K). The Ln[$(2e^2/h)\rho_{max}$] follows a linear dependence on B in the intermediate field range (10 T ~30 T), consistent with the plots in the inset of Fig. 3b The $\rho_{max}$ is observed to saturate toward ~$h/2e^2$ at even higher fields (>30 T, inset of Fig. S4b).

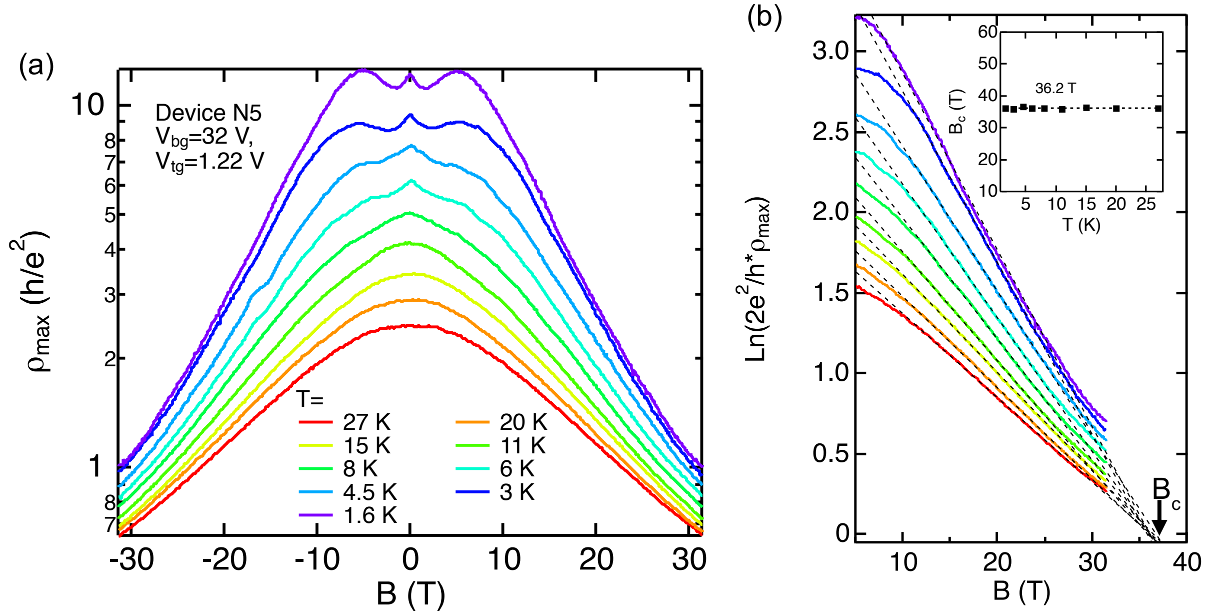


Fig. S5. (a) The measurements of $\rho_{max}$ (at fixed gate voltages) in Device N5 as a function of the in-plane magnetic field B in different temperatures in a third cool down. The highest field is 31.5 T. The $\rho_{max}$ in log

scale shows a linear dependence on B above a few T, with the corresponding plots of Ln[$(2e^2/h)\rho_{max}$] versus B in the positive field range shown in (b). All the linear fits (dashed lines) converge to a critical field $B_c$=36.2 T, with $B_c$ values for different curves extracted from the intercept on the B-axis plotted in the inset.

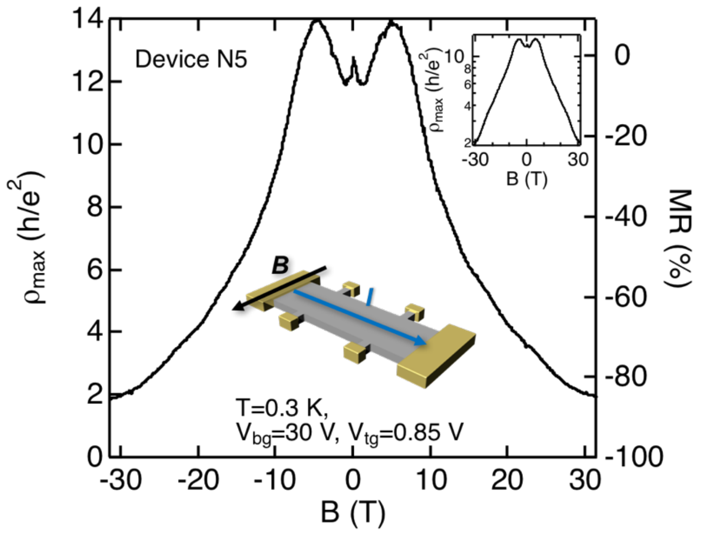


Fig. S6. The in-plane field dependence of $\rho_{max}$ (left axis) and the corresponding MR (right axis) for Device N5 in a configuration (schematic in the inset) with in-plane field (B) orthogonal to the current (I). The top right inset shows $\rho_{max}$ in log scale versus B.

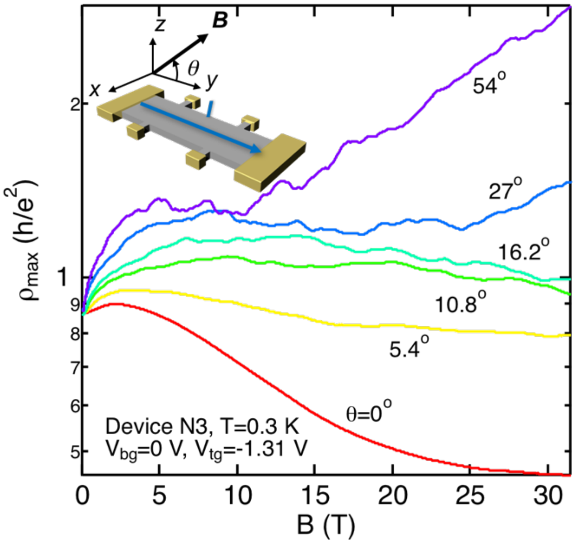


Fig. S7. The magnetic field dependence of $\rho_{max}$ for Device N3 with various angles between the magnetic field (in the yz plane) and the sample surface (the xy plane). The y-axis is along the current direction and z-axis is normal to the sample surface. The negative MR almost disappears with a small tilting angle $\theta \approx 10^o$, due to the out-of-plane component of the magnetic field.

According to the theory explained in part I and also in ref. [1], the negative MR has no requirement for the magnetic field direction as long as it is parallel to the surface (in-plane). In

Fig. S6, we showed the magnetotransport data of Device N5 in a configuration where the in-plane magnetic field is perpendicular to the current direction. In this case, we still observe a large negative MR above 5 T and it reaches -85% at 31 T. The residual resistivity ~2h/$e^2$ at 31 T is found to be higher comparing to ~h/$e^2$ in the parallel configuration (Fig. 2f) where a rotation probe is used (same for all other in-plane field measurements) and allows fine adjustment of angles (according to the minima in $R_{xx}$ and $|R_{xy}|$) to minimize the out-of-plane component. Typically, out-of-plane magnetic field induces *positive* MR (see an example of Device N3 in Fig. S7 while adjusting field direction relative to the sample plane). We note that the configuration used in this particular measurement (Fig. S6) could cause a small out-of-plane component of magnetic field due to imperfect alignment during sample mounting. This can partially explain the slightly higher resistivity at large fields comparing with the parallel-to-current configuration. More work may be needed to investigate if yet some other mechanisms can contribute to the small in-plane anisotropy.

## IV. Additional Data from Thicker Samples

In Fig. S8 and Fig. S9, we show more data on thicker (>$t_c$~10 nm) BSTS samples under in-plane magnetic fields. In these samples, only positive MR is observed.

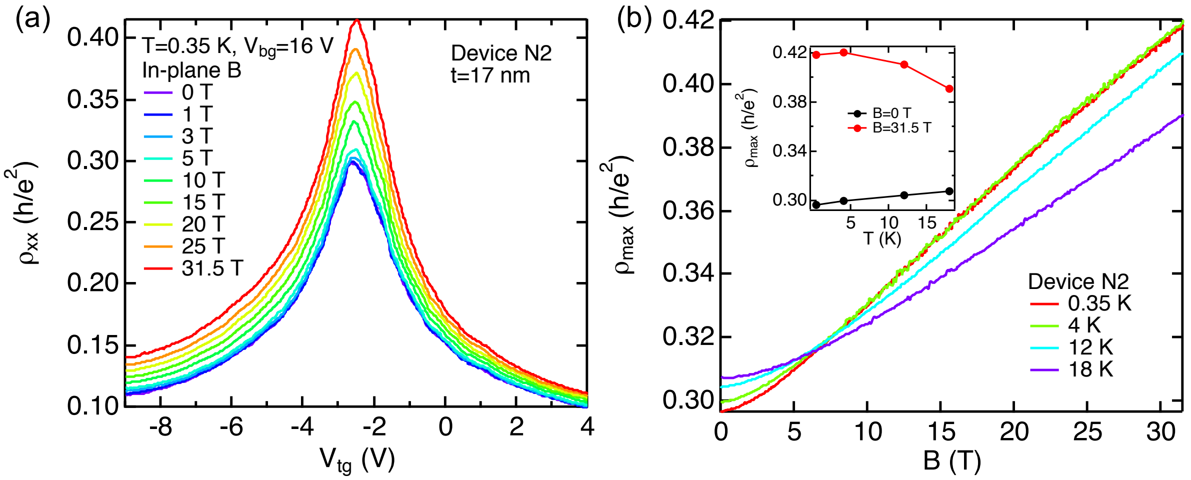


Fig. S8. (a) The raw data set for the 3D contour plot of Device N2 (17 nm thick gapless sample) in Fig. 3A, showing positive MR in the entire range of gate voltages. (b) The $\rho_{max}$ as a function of in-plane field at different temperatures for Device N2. The MR generally follows a $B^2$ dependence at low field and B dependence at higher field. With increasing B field, there is a crossover from the metallic to non-metallic

behavior (seen from the temperature dependence of the data at fixed fields, with two examples at 0 T and 31.5 T shown in the inset) at ~6 T.

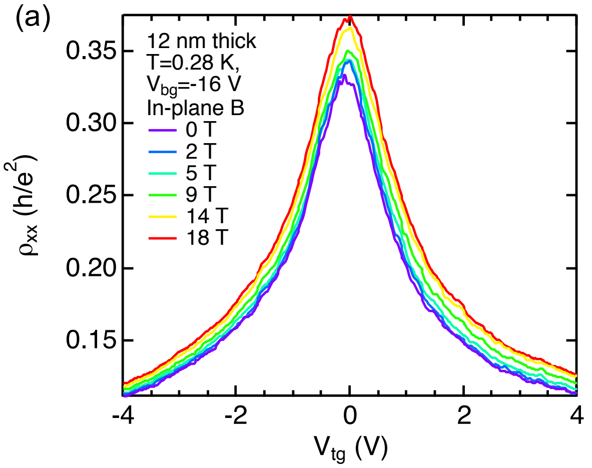


Fig. S9. Additional data showing the in-plane field effect on $\rho_{xx}$ of another (a) 12 nm thick and (b) 14 nm thick sample, showing only small positive MR in the range of gate voltages. Both are measured by tuning the top gate voltage through $\rho_{max}$ at fixed back gate voltages and base temperature (0.3 K).

SI References:


[1] A. A. Zyuzin, M. D. Hook, and A. A. Burkov, Phys. Rev. B **83**, 245428 (2011).

[2] Chang Liu, private communications.

[3] Y. Xu, I. Miotkowski, C. Liu, J. Tian, H. Nam, N. Alidoust, J. Hu, C.-K. Shih, M. Z. Hasan, and Y. P. Chen, Nat. Phys. **10**, 956 (2014).

[4] Y. Xu, I. Miotkowski, and Y. P. Chen, Nat. Commun. **7**, 11434 (2016).

[5] Y. Zhang, K. He, C.-Z. Chang, C.-L. Song, L.-L. Wang, X. Chen, J.-F. Jia, Z. Fang, X. Dai, W.-Y. Shan, S.-Q. Shen, Q. Niu, X.-L. Qi, S.-C. Zhang, X.-C. Ma, and Q.-K. Xue, Nat. Phys. **6**, 584 (2010).

[6] C.-X. Liu, H. Zhang, B. Yan, X.-L. Qi, T. Frauenheim, X. Dai, Z. Fang, and S.-C. Zhang, Phys. Rev. B **81**, 041307 (2010).

[7] J. Linder, T. Yokoyama, and A. Sudbø, Phys. Rev. B **80**, 205401 (2009).

[8] S. Cho, N. P. Butch, J. Paglione, and M. S. Fuhrer, Nano Lett. **11**, 1925 (2011).

[9] H. Z. Lu, W. Y. Shan, W. Yao, Q. Niu, and S. Q. Shen, Phys. Rev. B - Condens. Matter Mater. Phys. **81**, 115407 (2010).

[10] J. Liao, Y. Ou, X. Feng, S. Yang, C. Lin, W. Yang, K. Wu, K. He, X. Ma, Q. K. Xue, and Y. Li, Phys. Rev. Lett. **114**, 216601 (2015).

[11] I. Shlimak, E. Zion, A. V. Butenko, L. Wolfson, V. Richter, Y. Kaganovskii, A. Sharoni, A. Haran, D. Naveh, E. Kogan, and M. Kaveh, Phys. E Low-Dimensional Syst. Nanostructures **76**, 158 (2016).
